# Supplementary material for: Suppressed spontaneous emission for coherent momentum transfer
Source: arXiv:1903.01627 source file (2019-07-20)
Supplement: Supplementary file 1 [file supp.pdf]

# Supplementary materials for Suppressed spontaneous emission for coherent momentum transfer

Xueping Long, Scarlett S. Yu, Andrew M. Jayich, and Wesley C. Campbell

## COMB TOOTH EFFECTS

Due to the finite extinction ratio of the pulse picker (0.7%), small comb tooth effects can become important between pulse pairs during long pushing sequences. The quasi-steady-state scattering rate of an atom iluminated by a pulse train [1–3] can be used to assess how important comb tooth effects are, shown in Fig. S1 . At a pulse separation of 12.5 ns (80 MHz) intra-pulse coherence causes clear comb tooth effects in the calculated quasi-steady-state scattering rate (blue), whereas for 250 ns delay (40 MHz, red), the atomic response is nearly insensitive to comb tooth position (comb tooth visibility $V = 0.017$ [4]). For this work, we therefore operate the ML laser in the latter regime and away from resonance (gray shaded region) to avoid comb tooth effects. The passive stability of our laser is sufficient to maintain it in this regime, and we find that we do not need to use feedback to stabilize it.

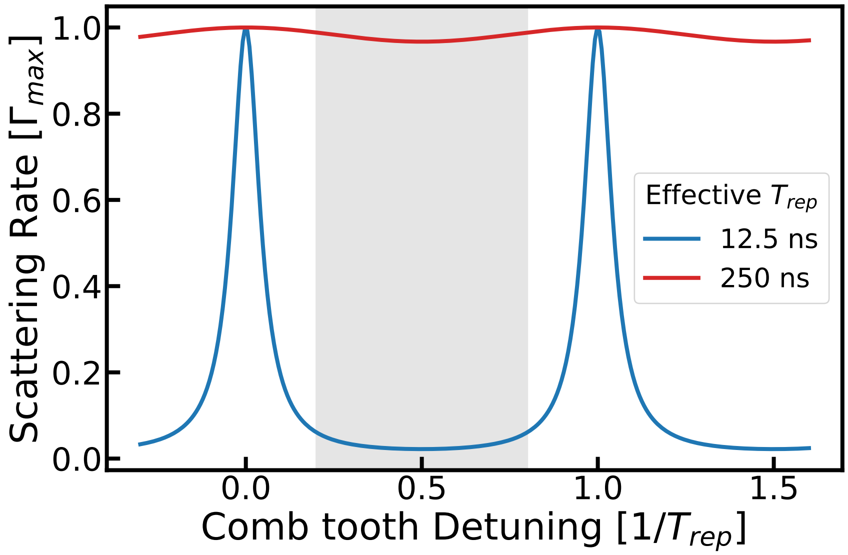


FIG. S1. Calculated quasi-steady-state normalized scattering rate for illumination by a ML pulse train. For the experiments in this work, the frequency comb was operated in the shaded region with respect to the blue curve.

## TIME OF FLIGHT MEASUREMENT

A resonant, cw laser beam centered 4 to 6 mm away from the initial position of the atomic cloud along the direction of the applied stimulated force is used to record absorption as a function of time for atoms accelerated by the pump-dump pulse pairs. The arrival times of the fastest 10% of the atoms (blue shaded area in Fig. S2 inset) are measured at 5 different TOF detection positions, shown in Fig. S2. The velocity of these atoms are obtained from a linear fit and converted to effective number of momentum transfers completed, giving rise to a momentum transfer efficiency of $91 \pm 3\%$.

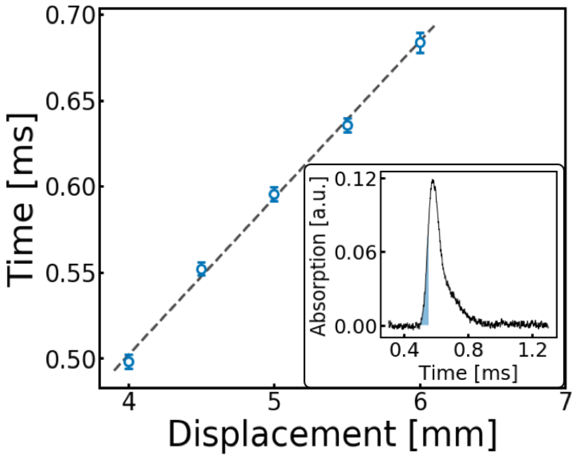


FIG. S2. Arrival times of the fastest 10% of the atoms at 5 different TOF detection positions, and the velocity fit (dashed line) obtained from the position and time data. The inset shows a TOF trace used to calculate the arrival time of the fastest 10% of the atoms with a 4.5 mm displacement from the initial atomic cloud position (blue shaded region).


[1] D. Felinto, C. Bosco, L. Acioli, and S. Vianna, Optics Communications **215**, 69 (2003).
[2] E. Ilinova, M. Ahmad, and A. Derevianko, Phys. Rev. A **84**, 033421 (2011).
[3] D. Aumiler and T. Ban, Phys. Rev. A **85**, 063412 (2012).
[4] M. Ip, A. Ransford, A. M. Jayich, X. Long, C. Roman, and W. C. Campbell, Phys. Rev. Lett. **121**, 043201 (2018).
